# Supplementary material for: Satellite to GroundScape -- Large-scale Consistent Ground View Generation from Satellite Views
Source: arXiv:2504.15786 source file (2025-04-22)
Supplement: Supplementary file 1 [file X_suppl.tex]

\clearpage
\setcounter{page}{1}
\maketitlesupplementary

In this supplementary material, we present further details on the methodology (\cref{sec:supp1}), provide comprehensive information about the dataset (\cref{sec:supp2}), report additional experimental results (\cref{sec:supp3}), and discuss the limitations of our approach (\cref{sec:supp4}).

\section{Additional methodology details}
\label{sec:supp1}
\subsection{Scene initialization and representation}
Our approach initializes the 3D scene in a format that prioritizes preserving the fidelity of the original satellite data, enabling effective camera control and ground-view generation. Unlike existing methods such as InfinitCity \cite{lin2023infinicity} and Sat2Scene \cite{Li_2024_CVPR}, which utilize sparse point clouds, we represent the scene as a unified triangle mesh \(\boldsymbol{M} = (\boldsymbol{V}, \boldsymbol{F}, \boldsymbol{E}, \boldsymbol{F}_{UV})\). This mesh consists of vertices (3D positions), faces, edges, and texture coordinates that define the appearance of each face, providing a denser and more comprehensive representation of the scene’s geometry, appearance, and visibility compared to sparse point clouds. We begin with a collection of satellite images \(\{\boldsymbol{I}^i\}\) and use traditional multi-view stereo (MVS) algorithms \cite{hirschmuller2005accurate} to generate depth maps \(\{\boldsymbol{D}^i\}\). These depth maps are projected and fused into 3D space to form an initial point cloud, \(\boldsymbol{P}_0\). Using the geometry refinement method described in \cite{xu2024geospecific}, \(\boldsymbol{P}_0\) is refined to \(\boldsymbol{P}_1\), which better captures building facades. The refined point cloud \(\boldsymbol{P}_1\) is then triangulated to produce the triangle mesh \(\boldsymbol{M} = (\boldsymbol{V}, \boldsymbol{F}, \boldsymbol{E})\). Finally, texture coordinates \(\boldsymbol{F}_{UV}\) are computed by mapping the satellite images \(\{\boldsymbol{I}^i\}\) onto \(\boldsymbol{M}\) using texture mapping techniques \cite{ling2023large}.

\subsection{Ground view foundation model}
Our framework is built upon a pre-trained LDM \cite{rombach2022high}, specifically leveraging a UNet-based architecture,  \(\epsilon_\theta\), trained on the large-scale text-image dataset LAION-5B \cite{schuhmann2022laion}. This model has demonstrated robust capabilities in generating high-fidelity images within the ground-view domain \cite{rombach2022high}. Our objective is to guide \(\epsilon_\theta\) effectively to synthesize ground-view images with layouts and appearances that accurately correspond to the input satellite views and their associated camera poses. To achieve this, we use \(\epsilon_\theta\) as a foundational model and integrate additional modules to bridge the domain gap between satellite and ground-view imagery.

\subsection{Network architecture}
We show the network architecture of satellite-guided denoising and satellite-temporal denoising process, \(\epsilon_{\theta}\), \(\mathcal{E}_{sat}\) and \(\epsilon_{\phi}\) in \cref{fig:supp_sat_archi}. The LDM \(\epsilon_{\theta}\) employs a standard UNet architecture. The \(\mathcal{E}_{sat}\) is designed to encode the satellite appearance \(\boldsymbol{I}_{g}\) using a combination of "CrossAttentionDownBlock", "DownBlock" and "CrossAttentionMidBlock". For satellite-temporal denoising module \(\epsilon_{\phi}\), we enhance the existing UNet structure by incorporating "TemporalResBlock" and "TemporalAttnBlock". The "TemporalResBlock" contains several 3D convolution layers, while the "TemporalAttnBlock" performs attention operations across the temporal axis (T) to achieve inter-frame learning. 
\begin{figure}
    \centering
    \begin{subfigure}[t]{0.5\linewidth}
        \includegraphics[width=\linewidth]{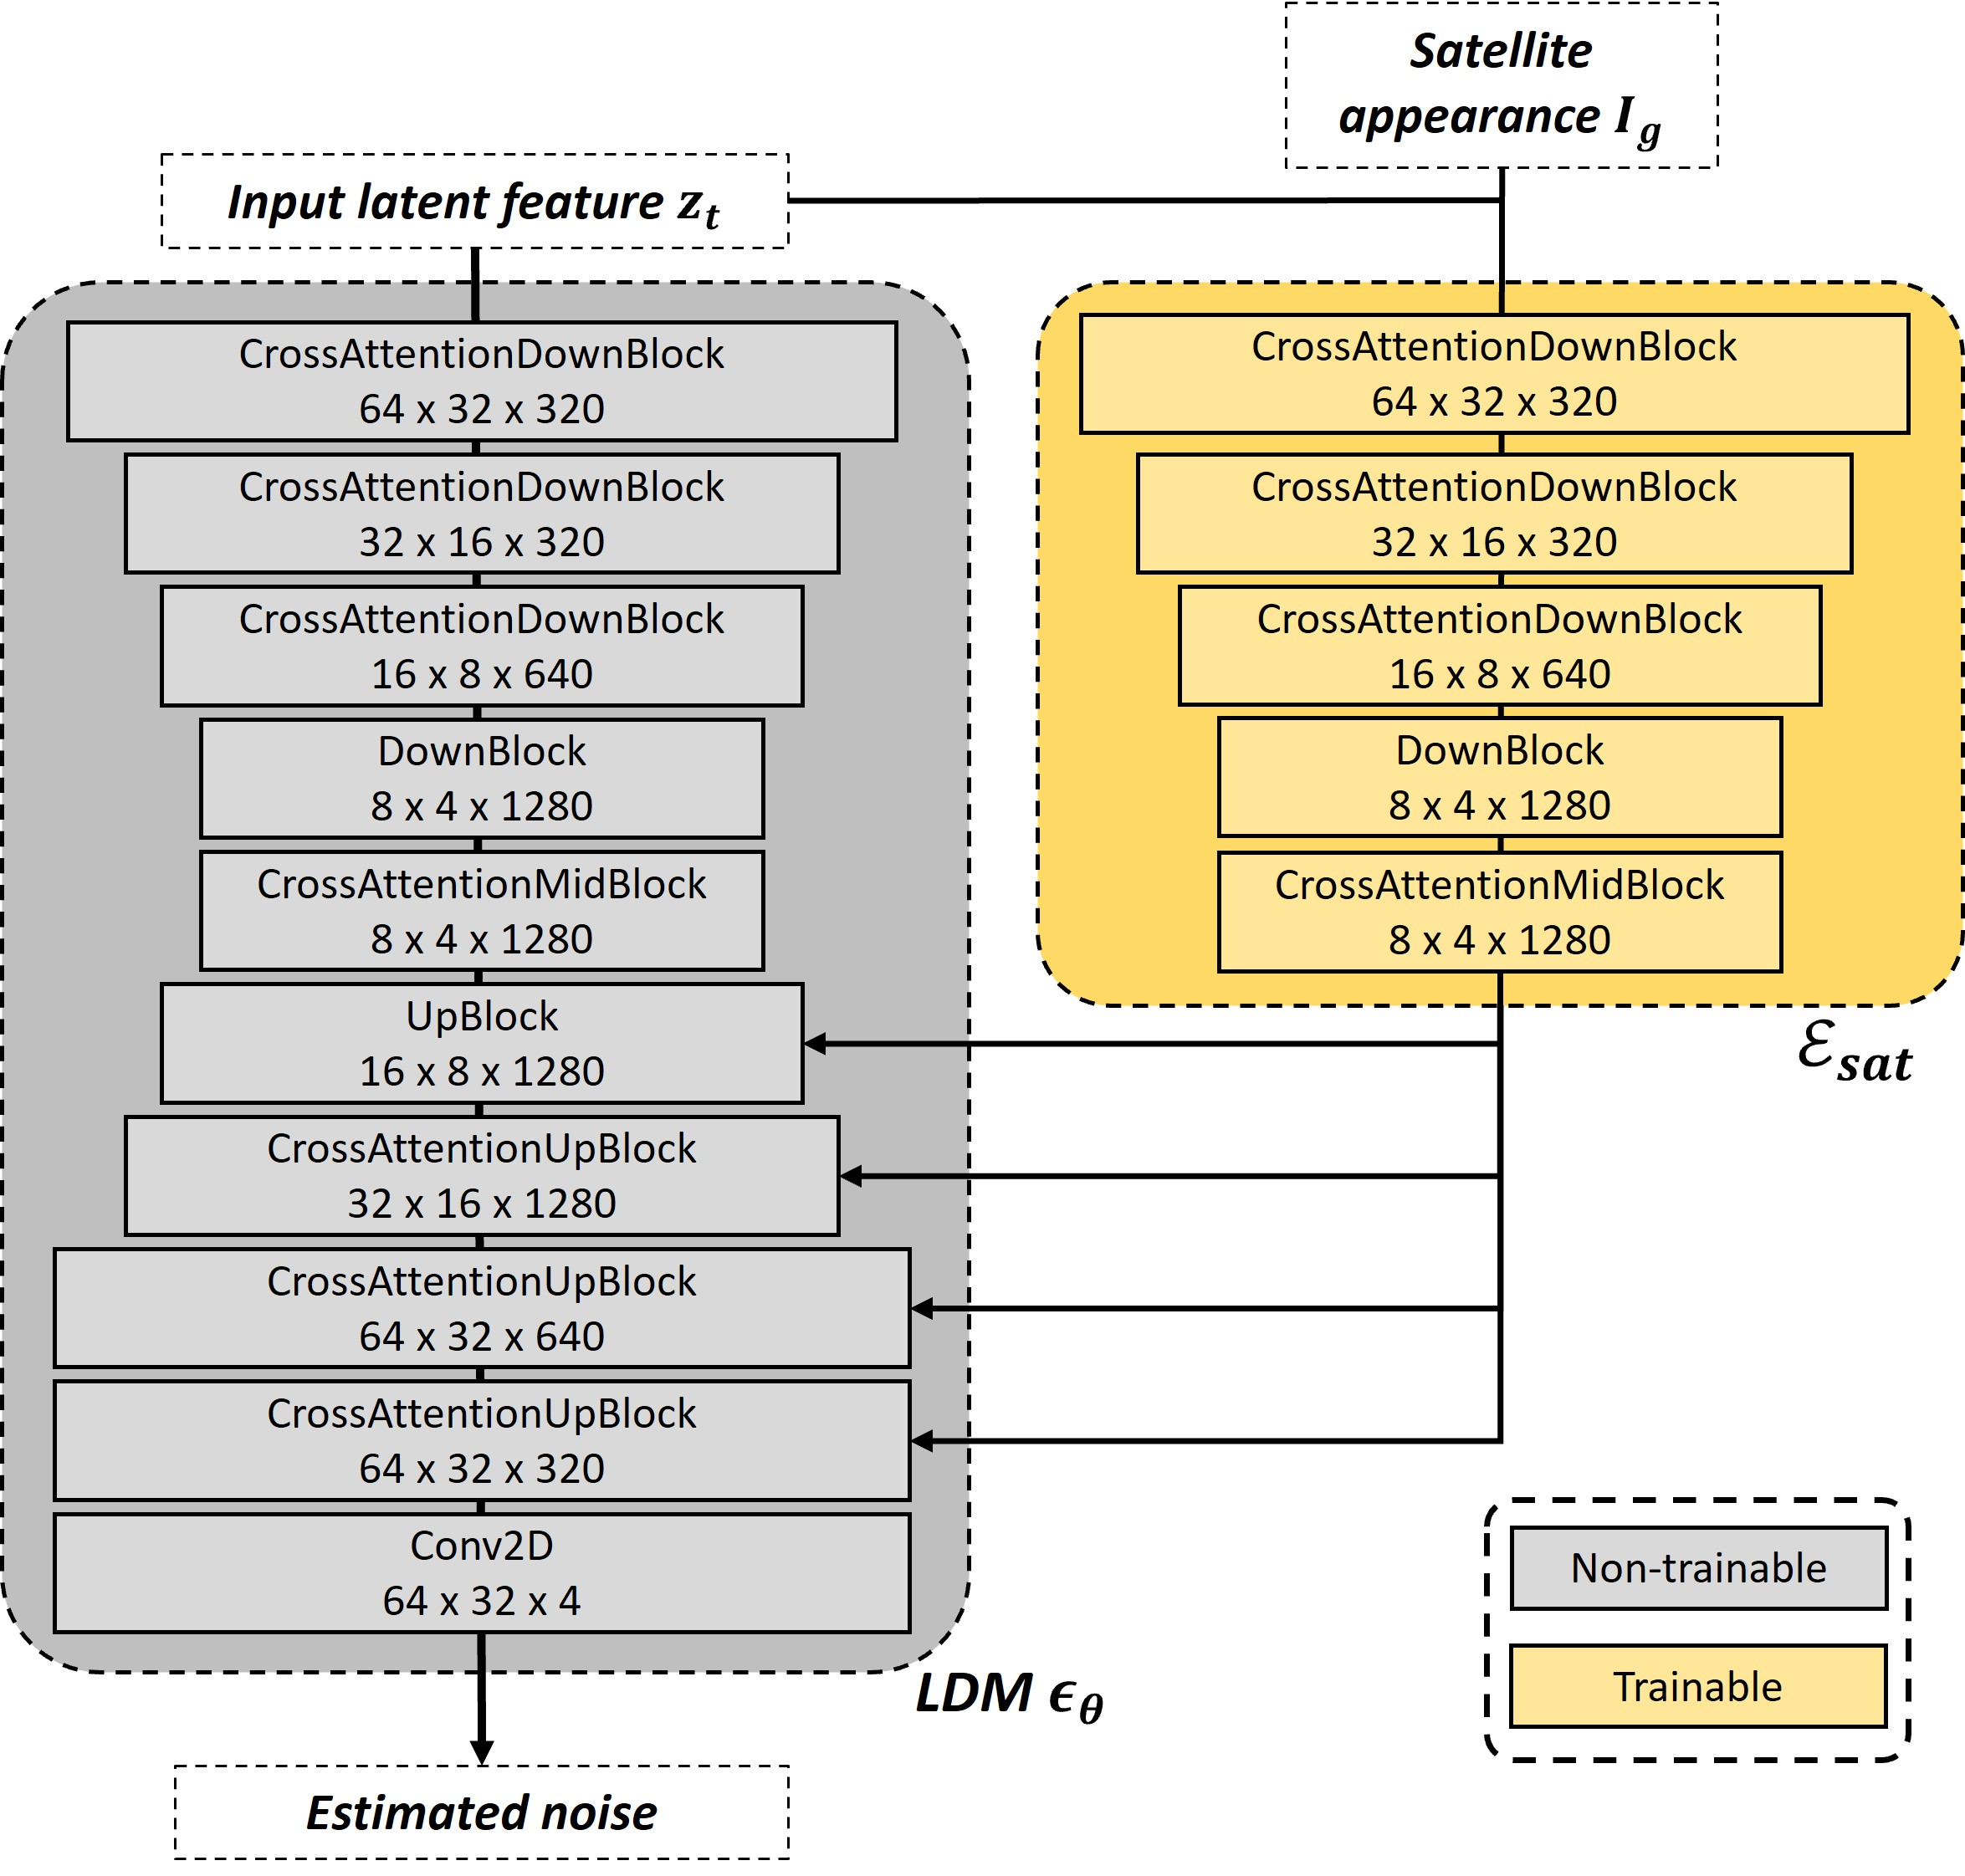}
        \caption{Architecture of \(\epsilon_{\theta}\) and \(\mathcal{E}_{sat}\)}
    \end{subfigure}
    \begin{subfigure}[t]{0.45\linewidth}
        \includegraphics[width=\linewidth]{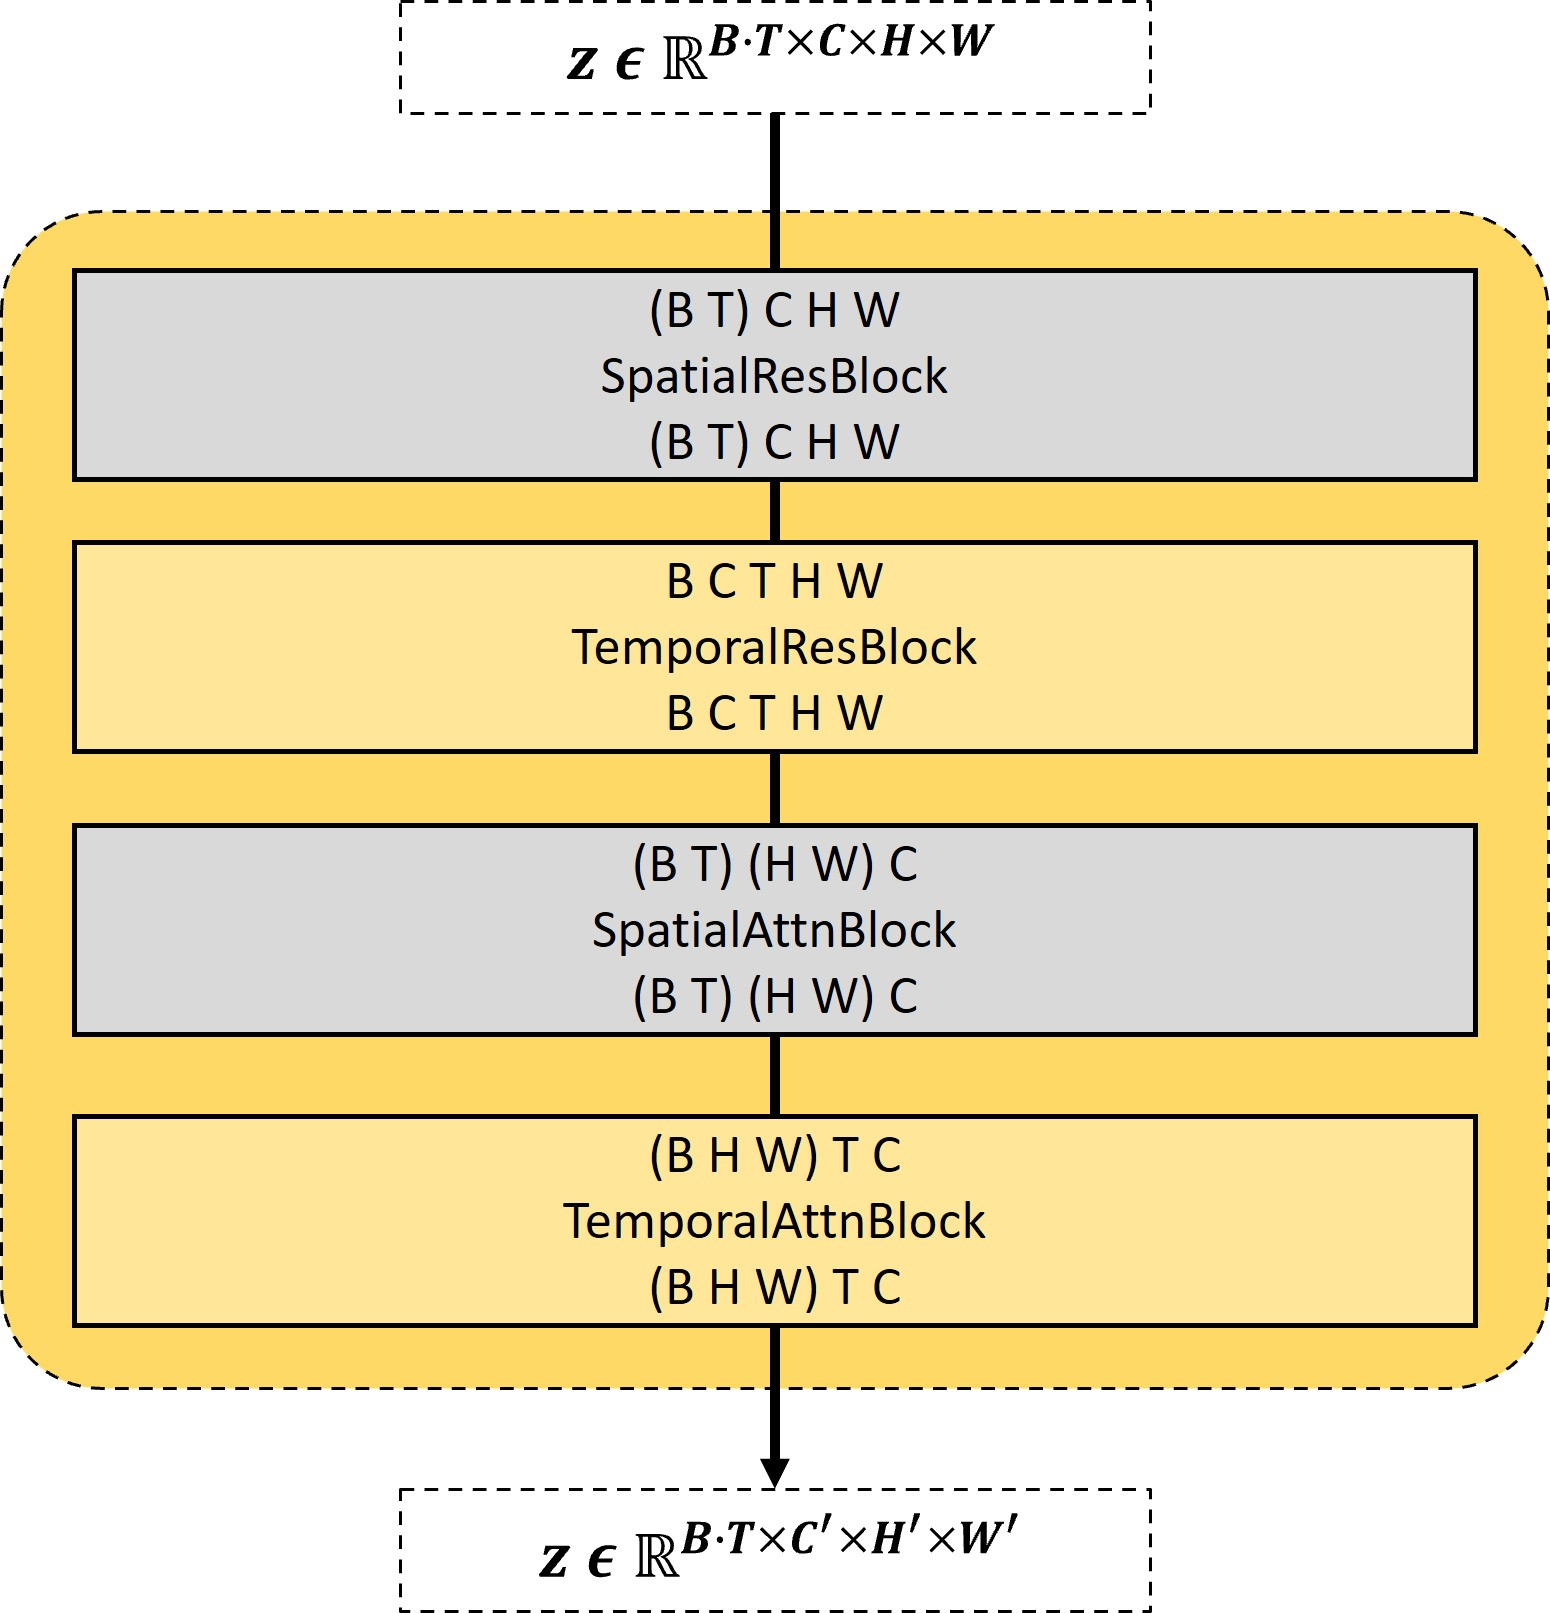}
        \caption{Architecture of a block of \(\epsilon_{\phi}\)}
    \end{subfigure}
    \caption{\textbf{Network architecture of \(\epsilon_{\theta}\), \(\mathcal{E}_{sat}\)} and \(\epsilon_{\phi}\). We provide detailed network architecture as the additional details to Fig. 3 \& Fig. 4 in the main manuscript.}
    \label{fig:supp_sat_archi}
\end{figure}
\subsection{Training \& inference}
The training process consists of two stages: in the first stage, \(\mathcal{E}_{sat}\) is trained using paired satellite appearance and ground truth images over 50,000 iterations with a batch size of 32. This stage enables \(\mathcal{E}_{sat}\) to extract high-level scene layout information to guide the LDM. In the second stage, \(\mathcal{E}_{\phi}\) and \(\epsilon_{\phi}\) are trained on paired sequences of five satellite appearance views and their corresponding ground truth over 100,000 iterations with a batch size of 12. This stage allows \(\mathcal{E}_{\phi}\) and \(\epsilon_{\phi}\) to learn the motion and temporal features. The inference process involves satellite-conditioned and temporal-conditioned denoising, as detailed in Sec. 3.3. We adopt the deterministic sampling process from DDIM \cite{song2020denoising} with 20 denoising steps under the classifier-free guidance framework \cite{ho2022classifier}.

\section{Additional dataset details}
\label{sec:supp2}
\subsection{Ground data processing}
The raw ground data is obtained via the GoogleStreetView API, which provides panoramic images at a resolution of 1024x2048, along with 3D location (longitude, latitude, elevation), and horizontal orientation (heading angle). The transformation process for converting each panoramic image into perspective views is detailed using camera intrinsic and extrinsic parameters. We define each perspective view within a panorama using the parameters \(\theta\), \(\phi\), \(FOV,H,W\). Here, \(\theta \in [0,360]\), and \(\phi \in [-90,90]\) specify the orientation of the perspective image in azimuth and altitude angles, respectively. \(FOV\) denotes the field of view, which implicitly determines the focal length, \(H\), and \(W\) represent the height and width of the perspective image. Specifically, we resample the “LR,” “LF,” “RF,” and “RR” perspective images for each panorama using the parameters \(\theta=[60,120,240,300]\), \(\phi=15\), \(FOV=75, H=256, W=256\).

\begin{figure}
    \centering
    \includegraphics[width=\linewidth]{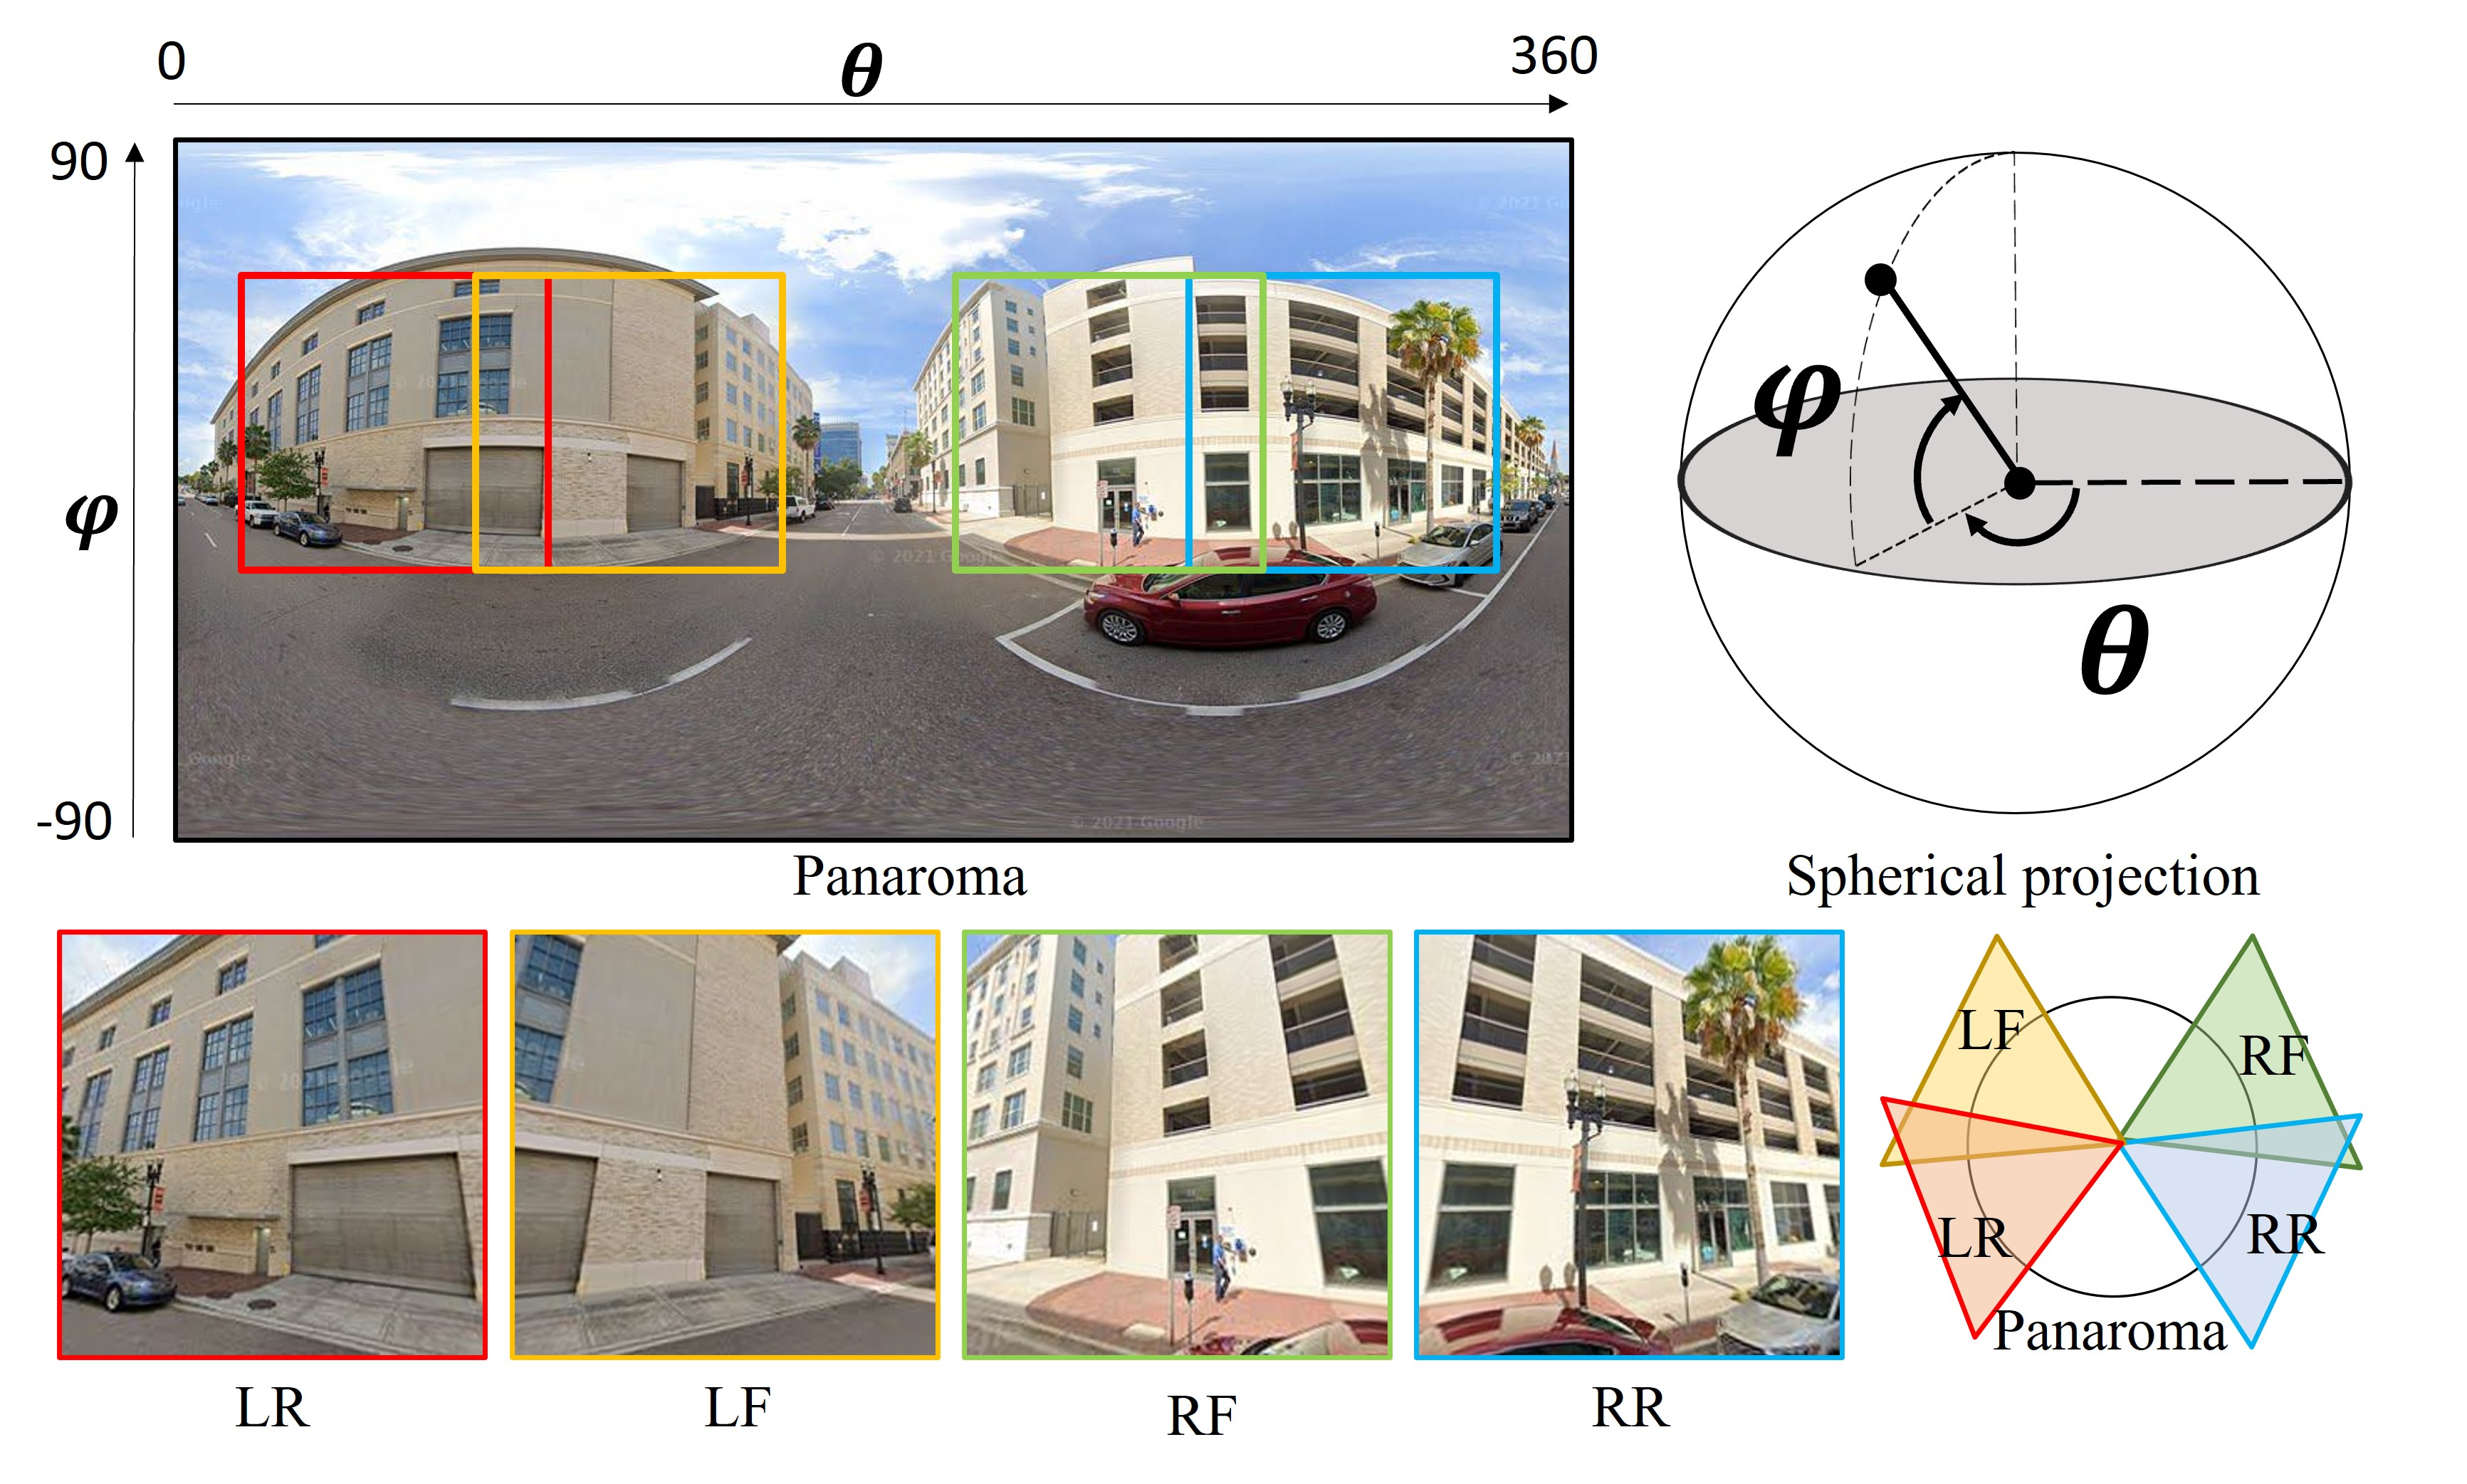}
    \caption{\textbf{Panaroma to perspective views.} The raw ground data is provided in panoramic format, where the coordinates of each pixel are defined by \(\theta\) and \(\phi\) in spherical projection. Each perspective view is resampled from a region of the spherical surface within \([\theta_{min},\theta_{max}],[\phi_{min},\phi_{max}]\).}
    \label{fig:supp_pana}
\end{figure}

\subsection{Train \& test data split}
The dataset spans a total area of \(130 KM^2\), divided into 90 tiles, each covering a \(600 \times 600\) region, as illustrated in \cref{fig:supp_coverage}. For fair evaluation, the tiles are partitioned into training and testing sets in a 70/20 ratio.

\begin{figure}
    \centering
    \includegraphics[width=\linewidth]{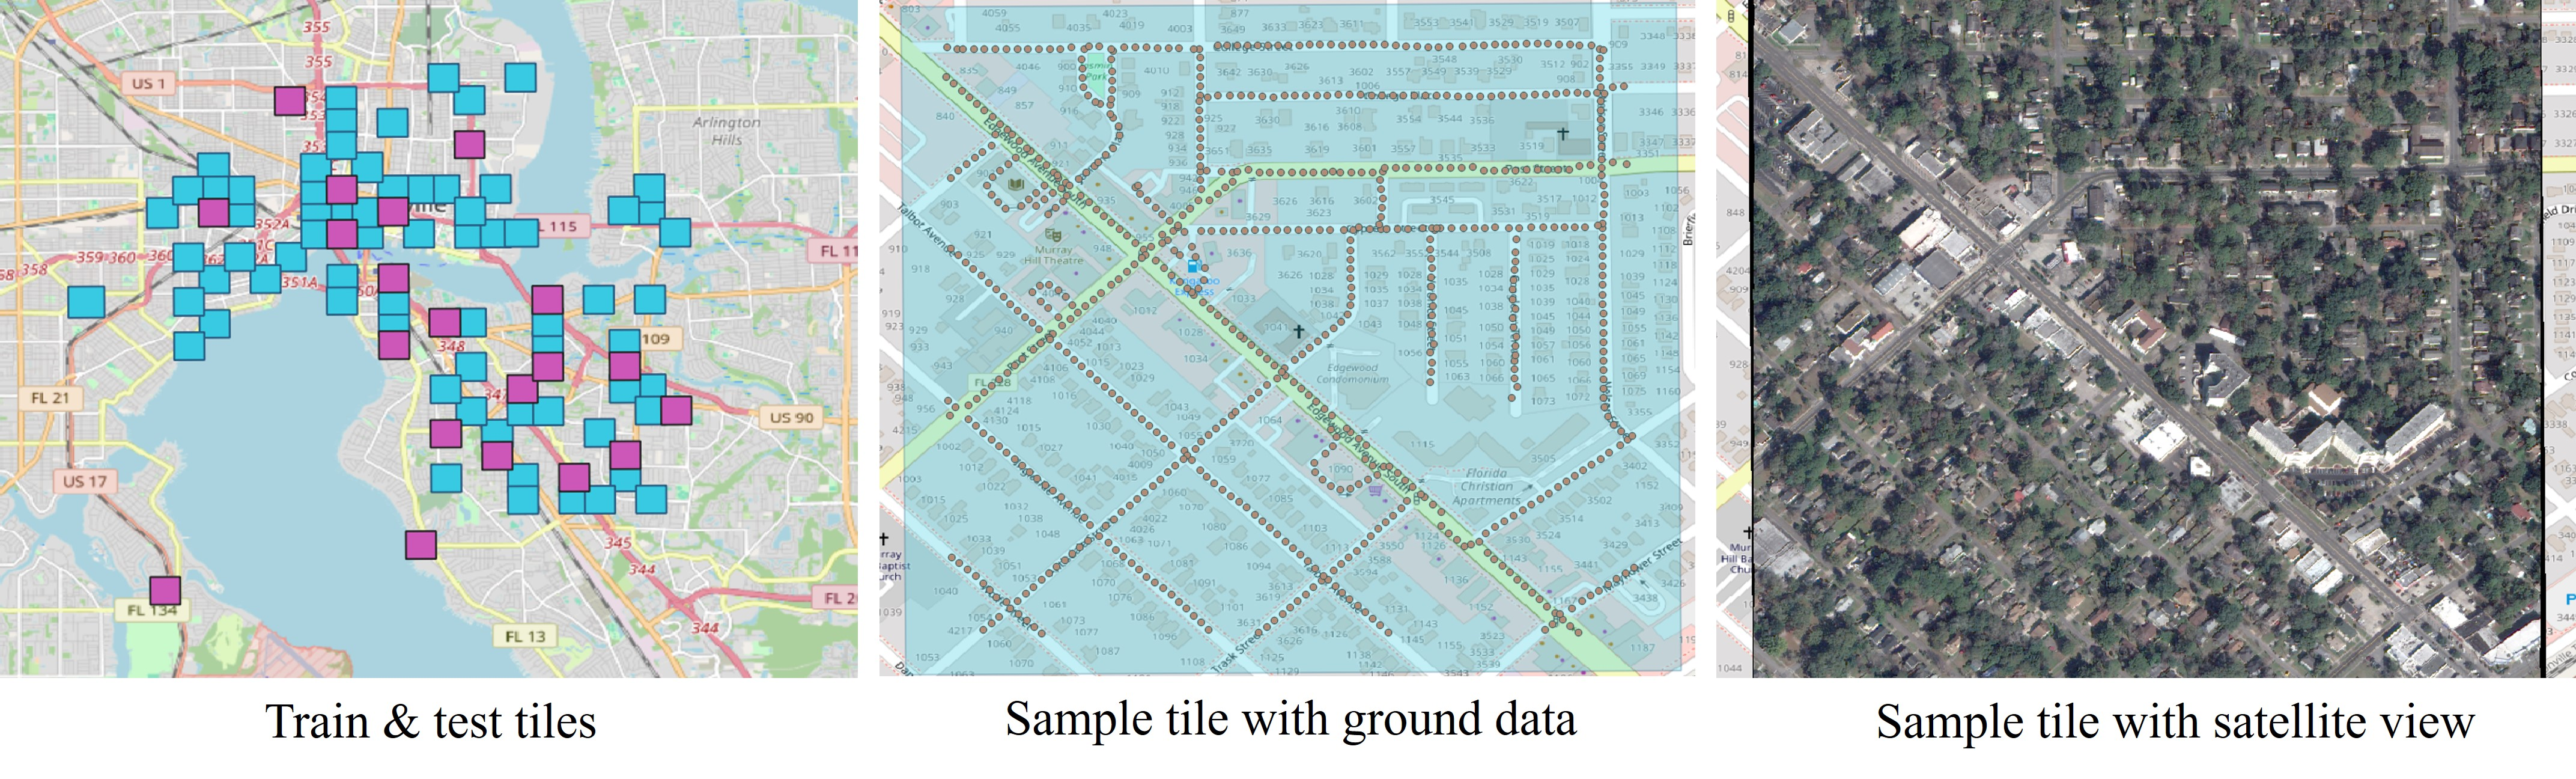}
    \caption{\textbf{Train \& test data split.} The data is split into training and testing sets based on tiles, with each tile covering a \(600 \times 600\) m area. A total of 90 tiles are used, with 70 tiles designated for training (in blue) and 20 tiles for testing (in pink).}
    \label{fig:supp_coverage}
\end{figure}
\section{Additional experiment results}
\label{sec:supp3}
Additional qualitative baseline comparisons are presented in \cref{fig:supp_quali}, serving as an extension of Fig. 6 in the main manuscript. The results demonstrate that our method consistently generates photorealistic ground views that maintain coherence across neighboring perspectives.

\section{Limitation}
\label{sec:supp4}
Although Sat2GroundScape generates photorealistic ground views with strong multi-view consistency, it has certain limitations, as illustrated in \cref{fig:supp_limit}. When satellite views provide insufficient appearance information, such as in shadowed or textureless regions, the \(\mathcal{E}_{sat}\) module in the satellite-guided denoising process is unable to extract useful features for ground view generation, resulting in random ground layouts or appearances. This limitation also affects the satellite-temporal denoising process, leading to inconsistencies across the entire sequence of ground views.

\begin{figure}
    \centering
  \begin{subfigure}[t]{\linewidth}
    \includegraphics[width=\linewidth]{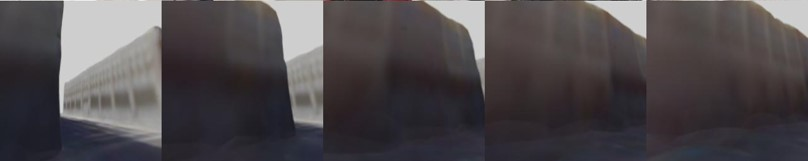}
    \caption{Satellite appearance}
  \end{subfigure}
        \begin{subfigure}[t]{\linewidth}
        \includegraphics[width=\linewidth]{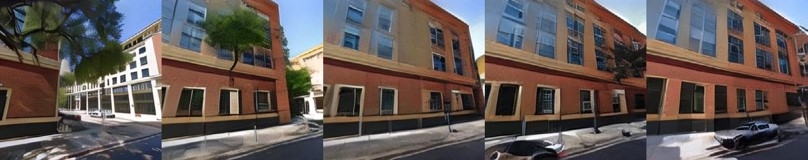}
        \caption{Ours}
    \end{subfigure}
        \begin{subfigure}[t]{\linewidth}
        \includegraphics[width=\linewidth]{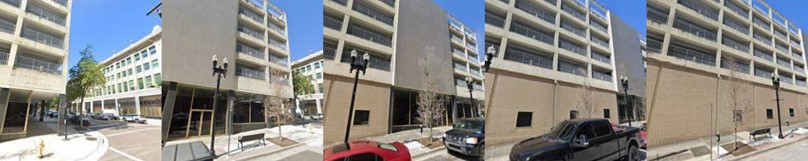}
        \caption{Ground truth}
    \end{subfigure}
    \caption{\textbf{Limitation}. In shadow regions, our satellite-guided denoising process struggles to extract meaningful texture features for the initial ground view generation, leading to incorrect textures and facade layouts. Furthermore, the erroneous initial ground view affects the generation of subsequent views in the sequence.}
    \label{fig:supp_limit}
\end{figure}

\begin{figure*}
    \centering
  \begin{subfigure}[t]{0.9\linewidth}
    \includegraphics[width=\linewidth]{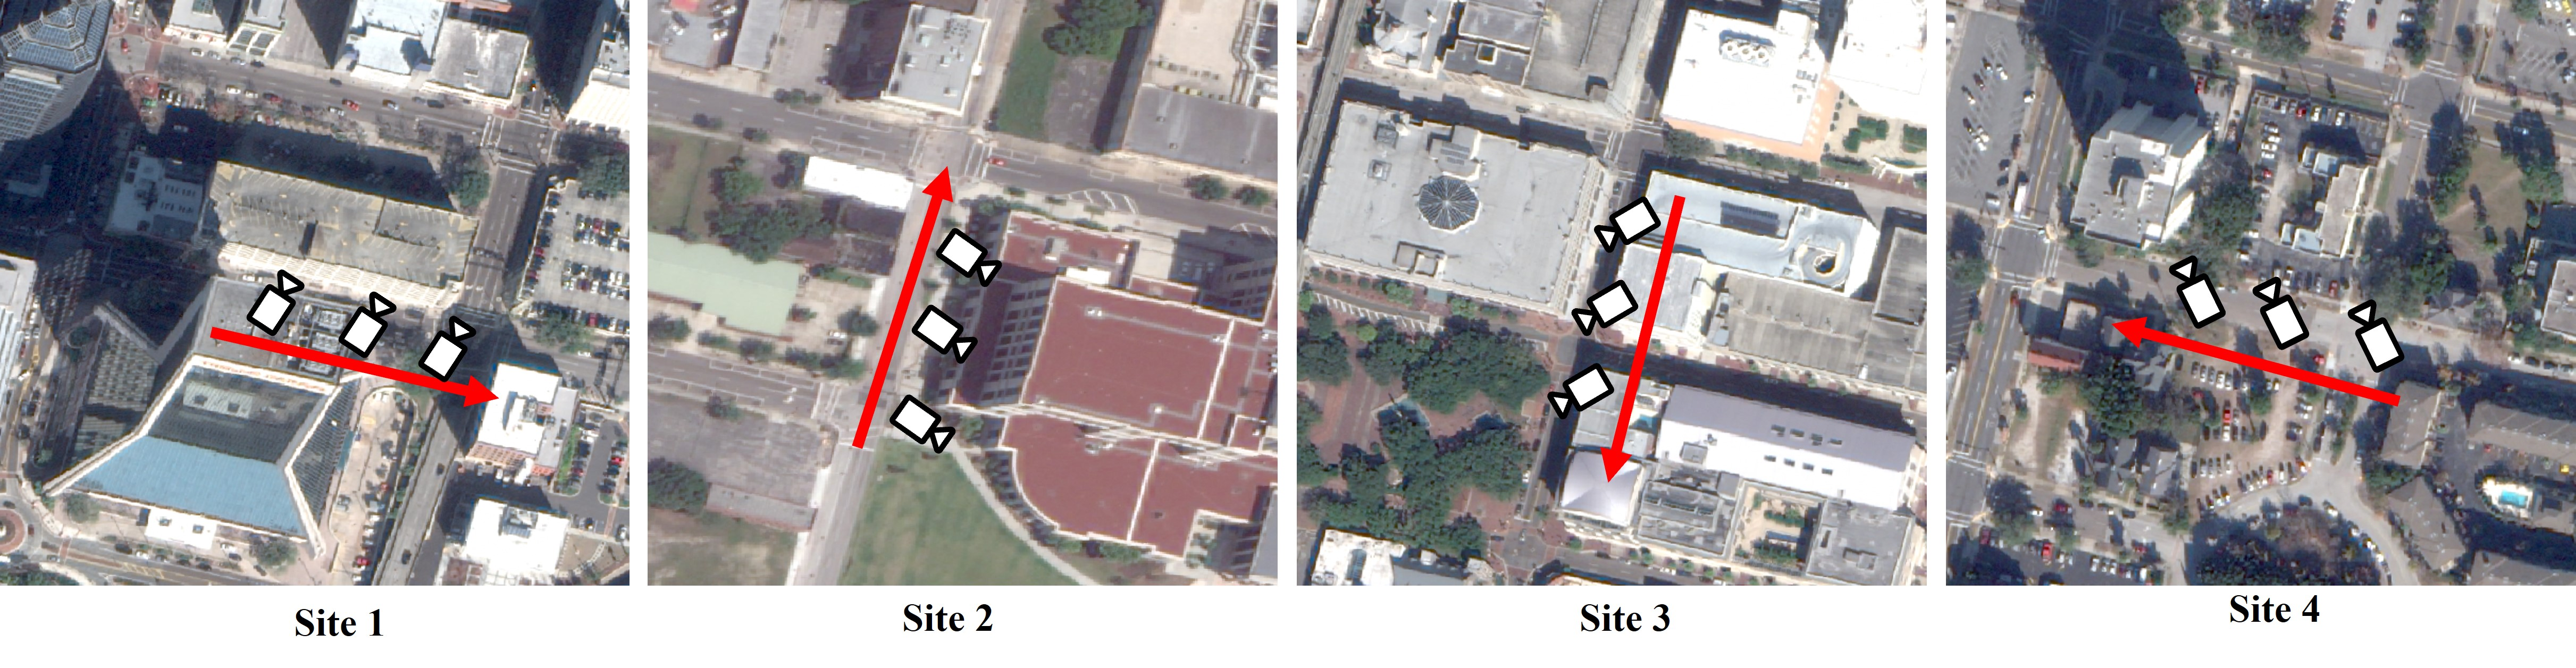}
    \caption{Satellite \& cameras}
  \end{subfigure}
    \begin{subfigure}[t]{0.47\linewidth}
    \includegraphics[width=\linewidth]{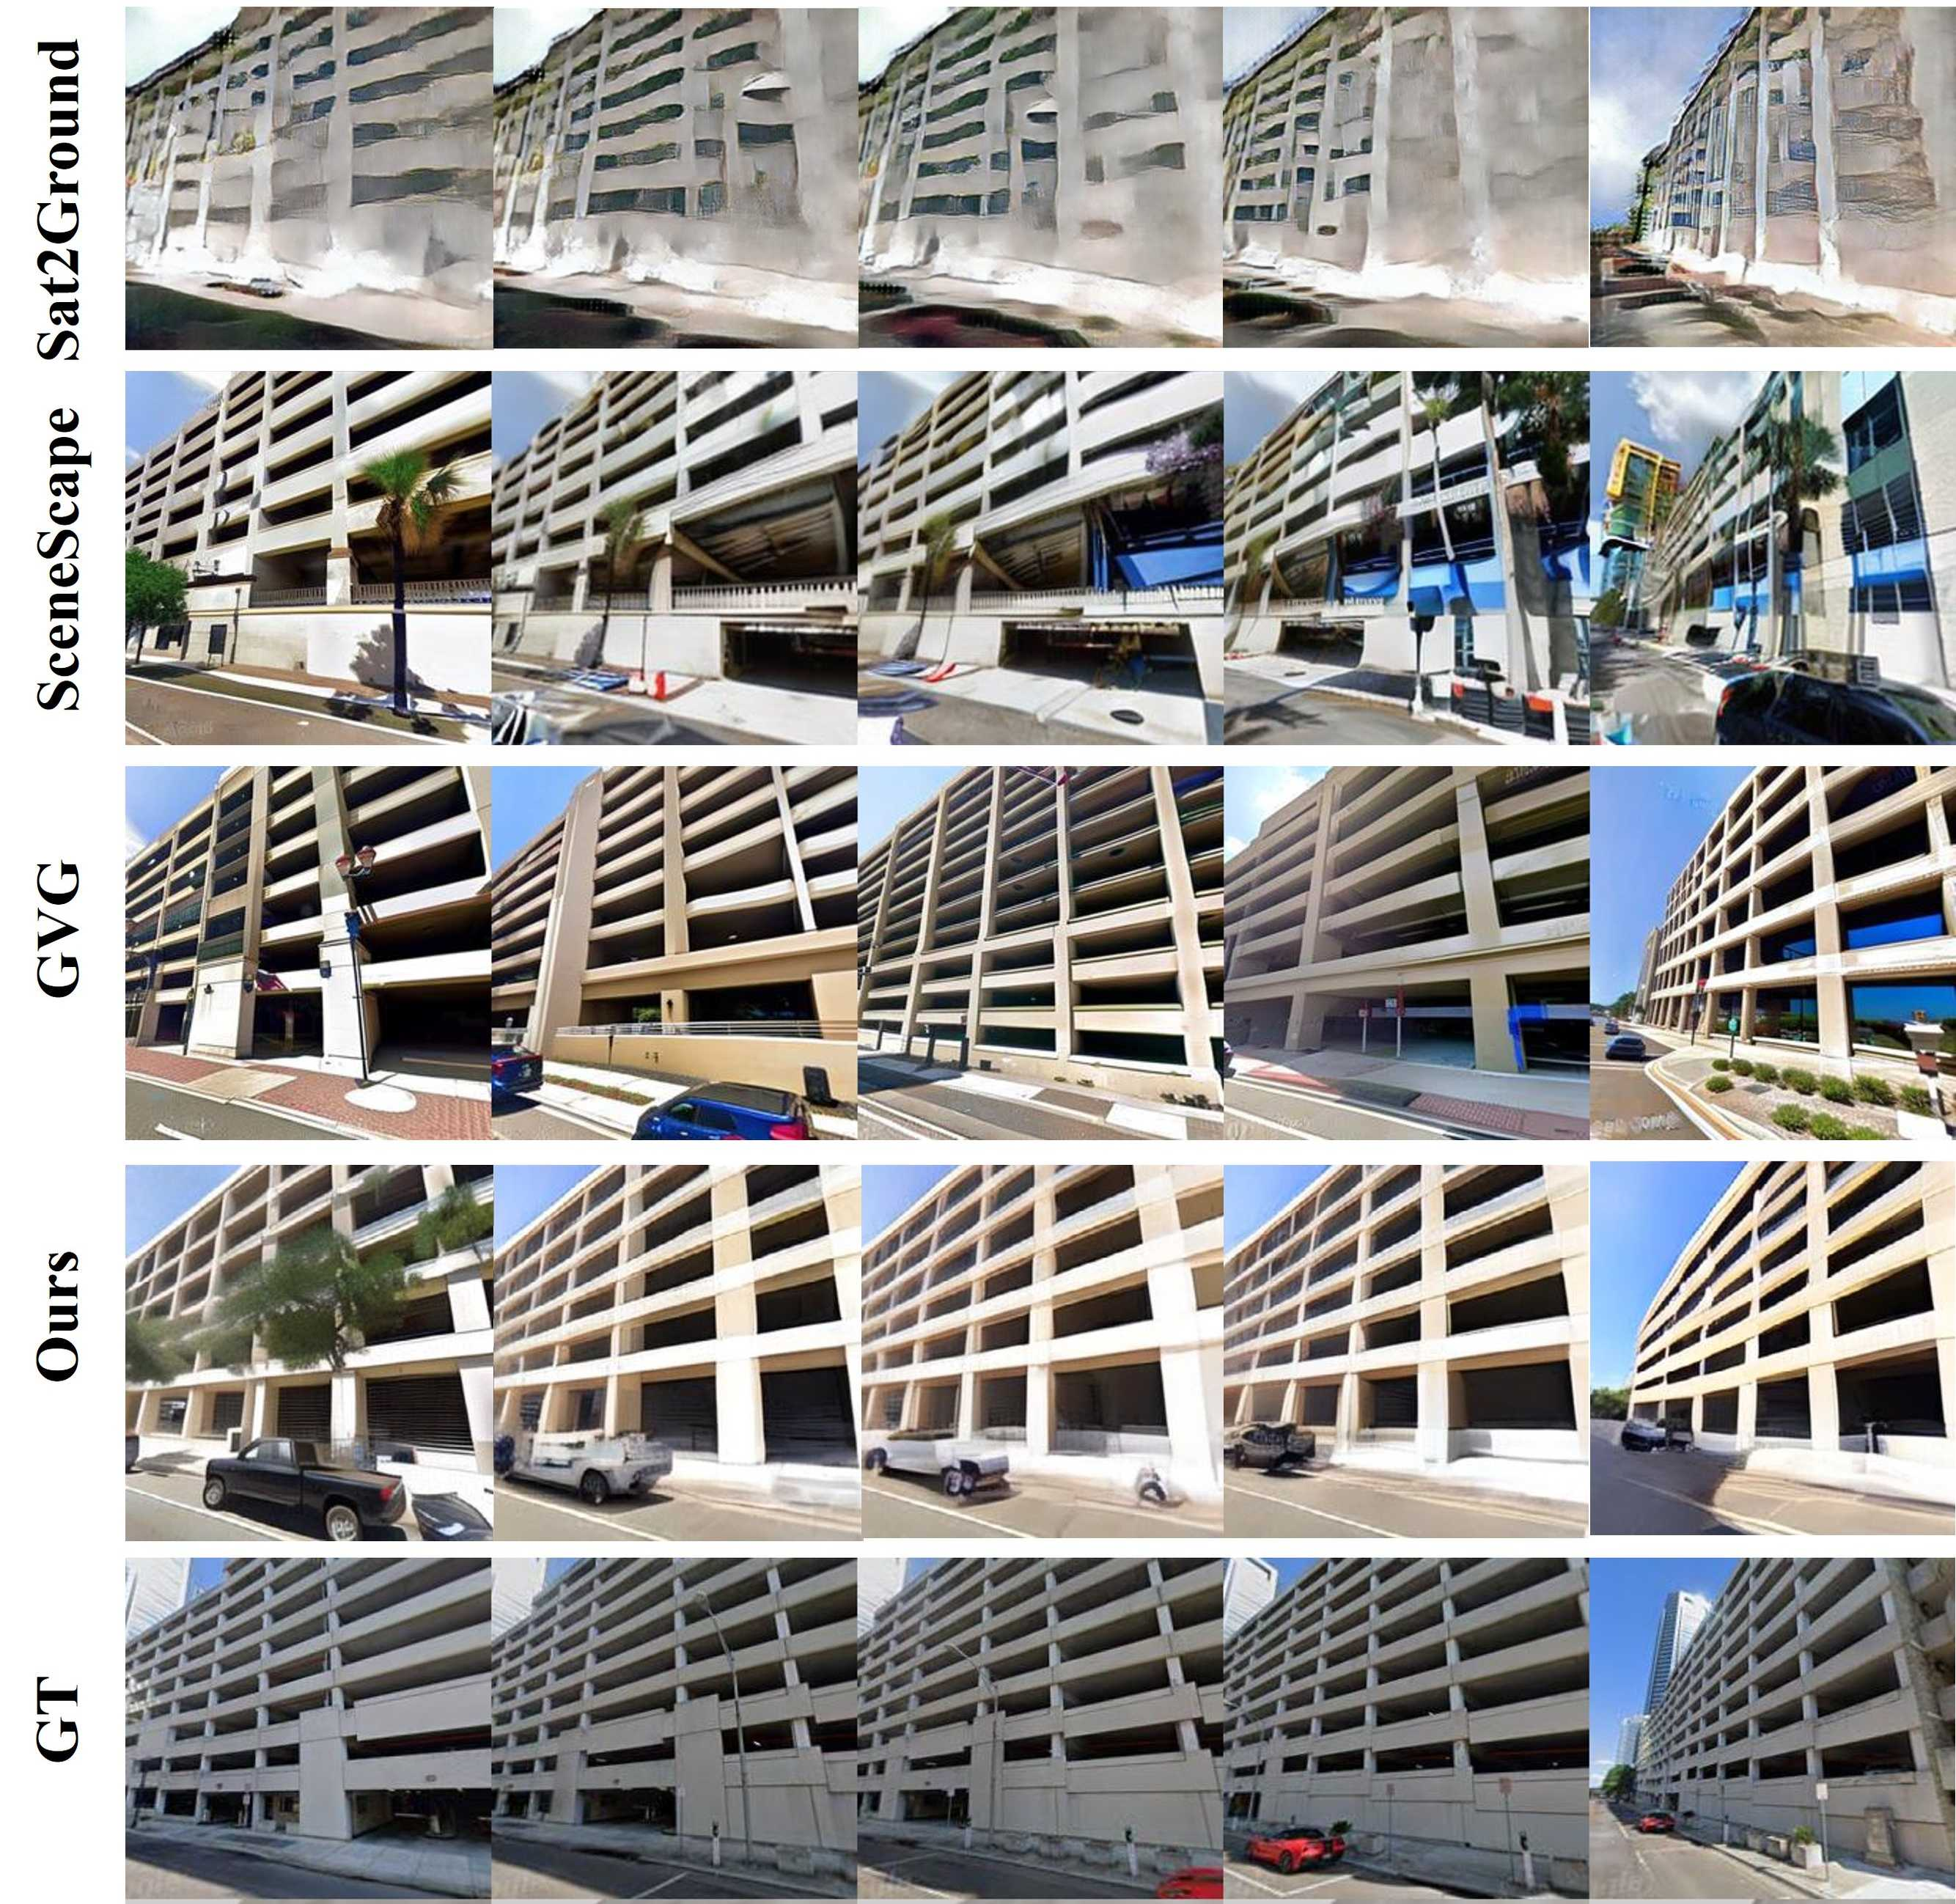}
    \caption{Site 1}
  \end{subfigure}
      \begin{subfigure}[t]{0.44\linewidth}
    \includegraphics[width=\linewidth]{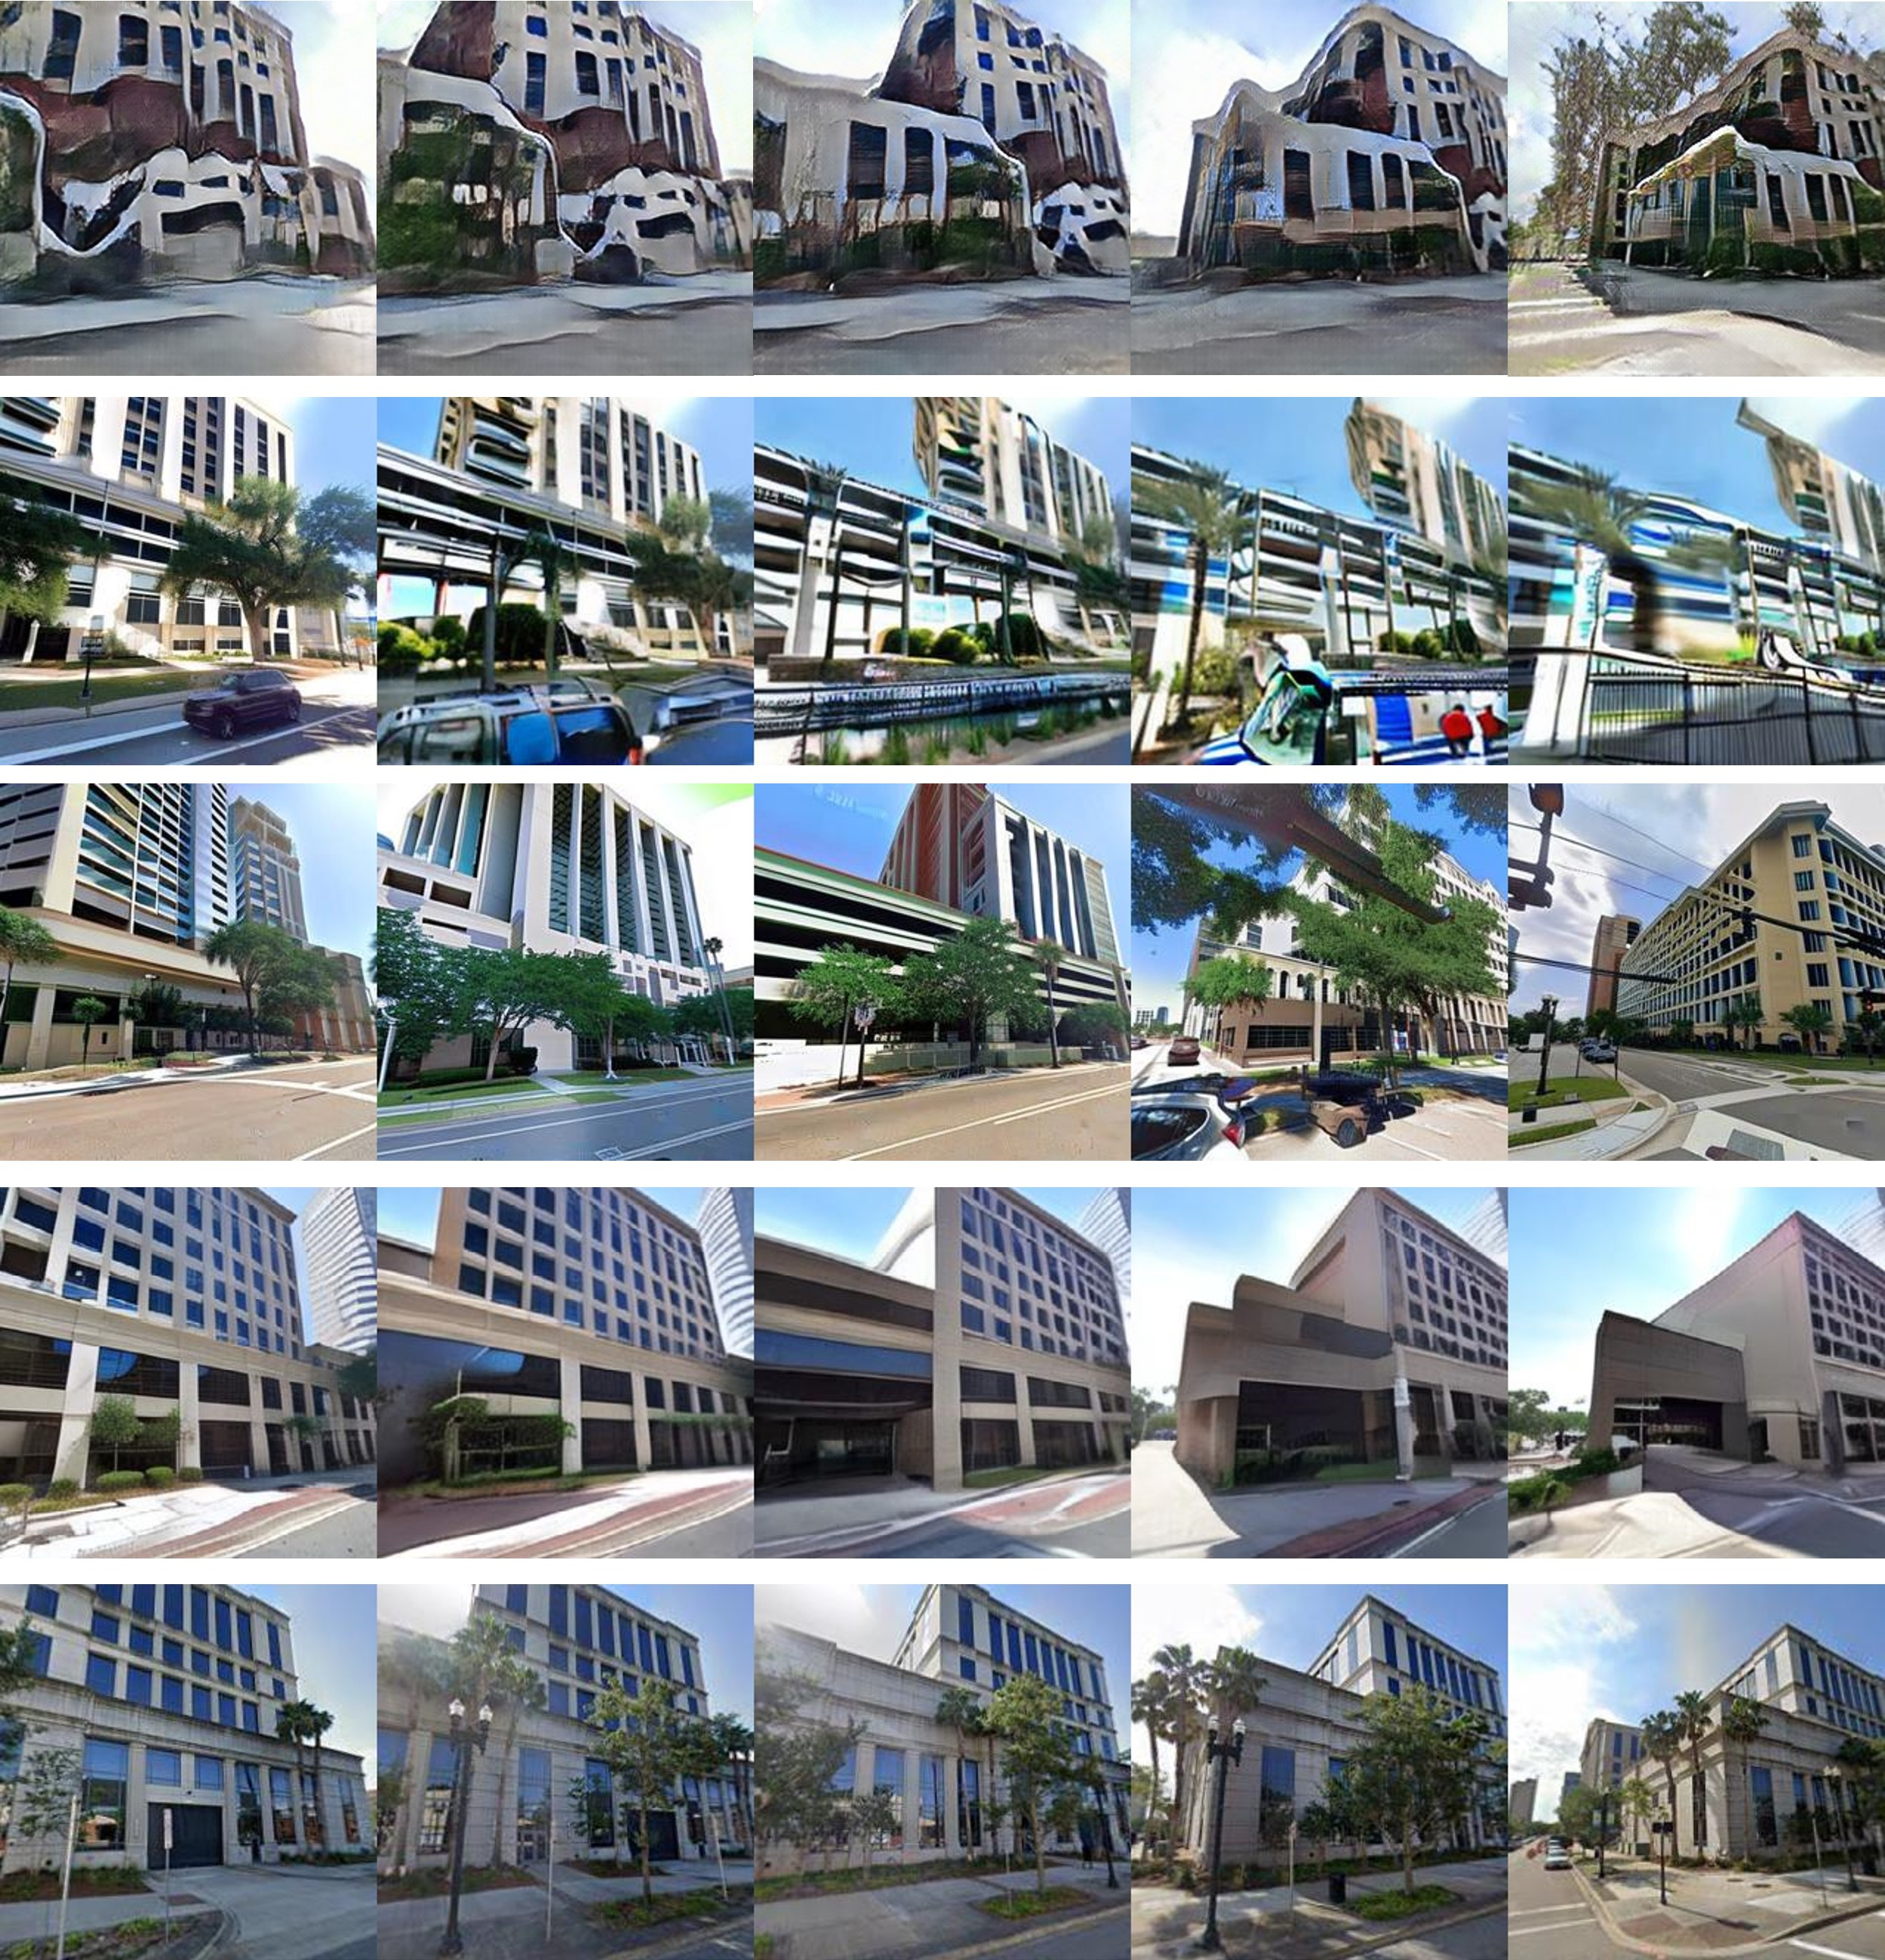}
    \caption{Site 2}
  \end{subfigure}
      \begin{subfigure}[t]{0.47\linewidth}
    \includegraphics[width=\linewidth]{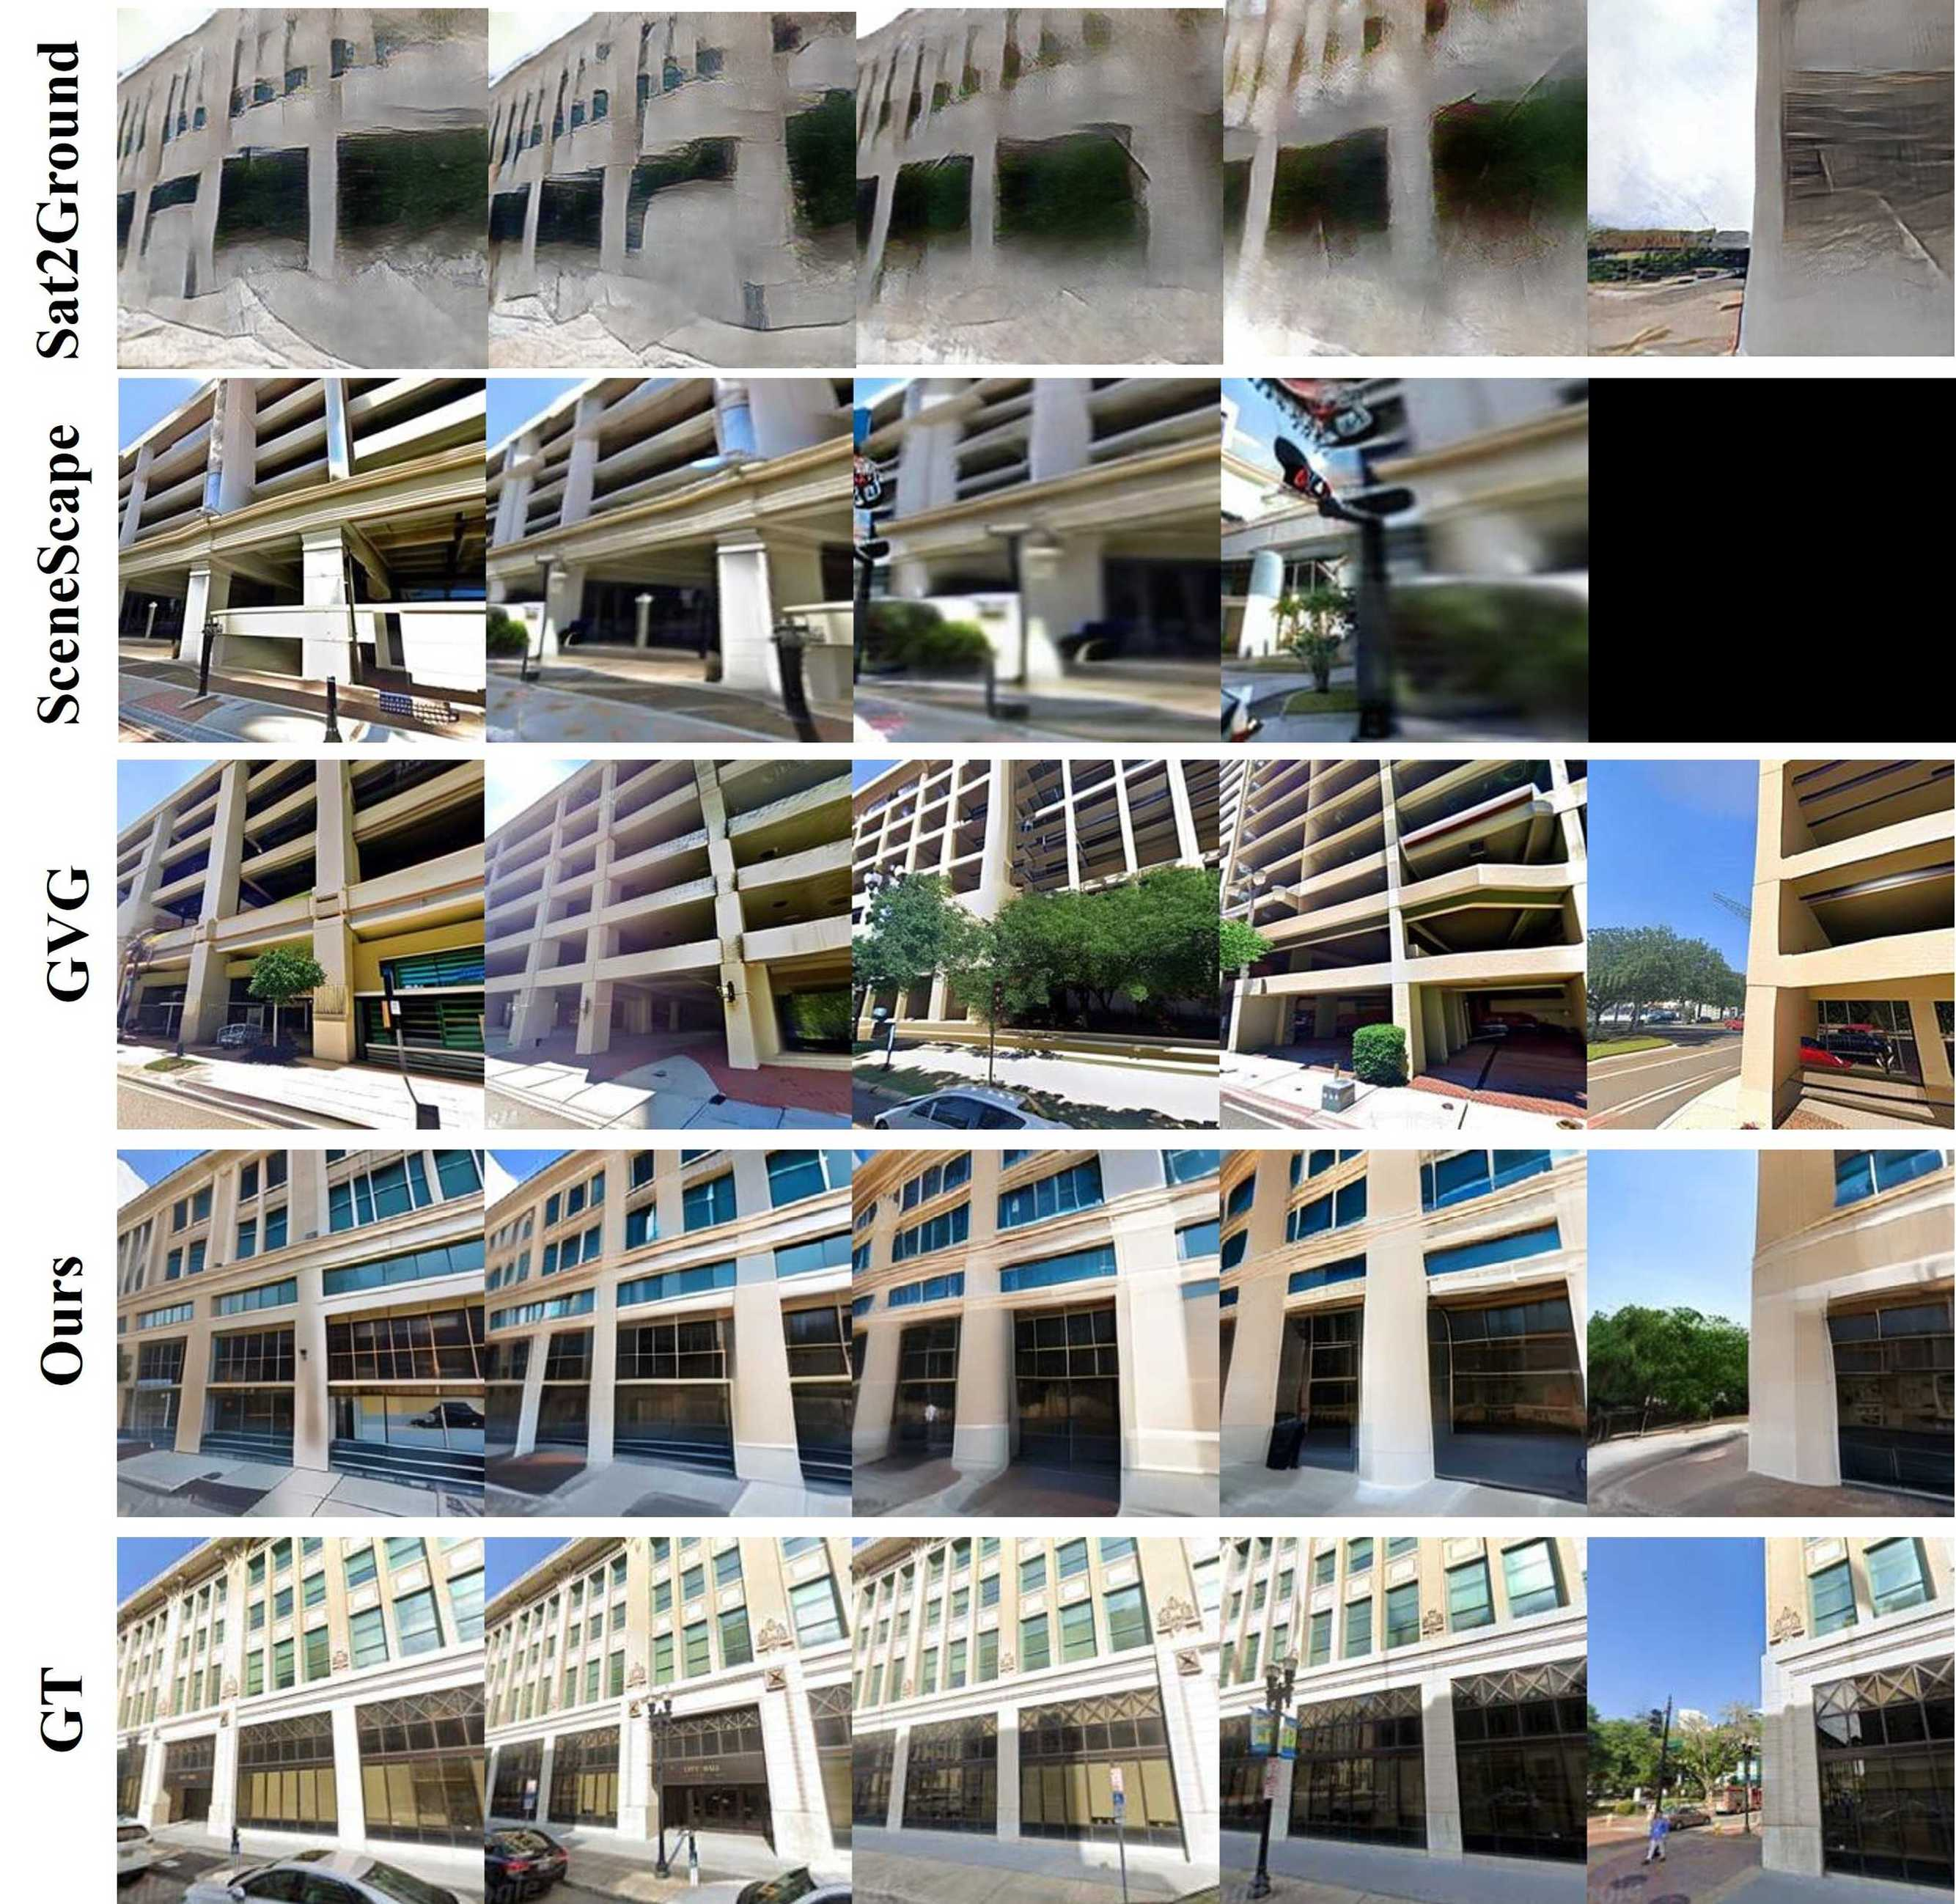}
    \caption{Site 3}
  \end{subfigure}
  \begin{subfigure}[t]{0.44\linewidth}
    \includegraphics[width=\linewidth]{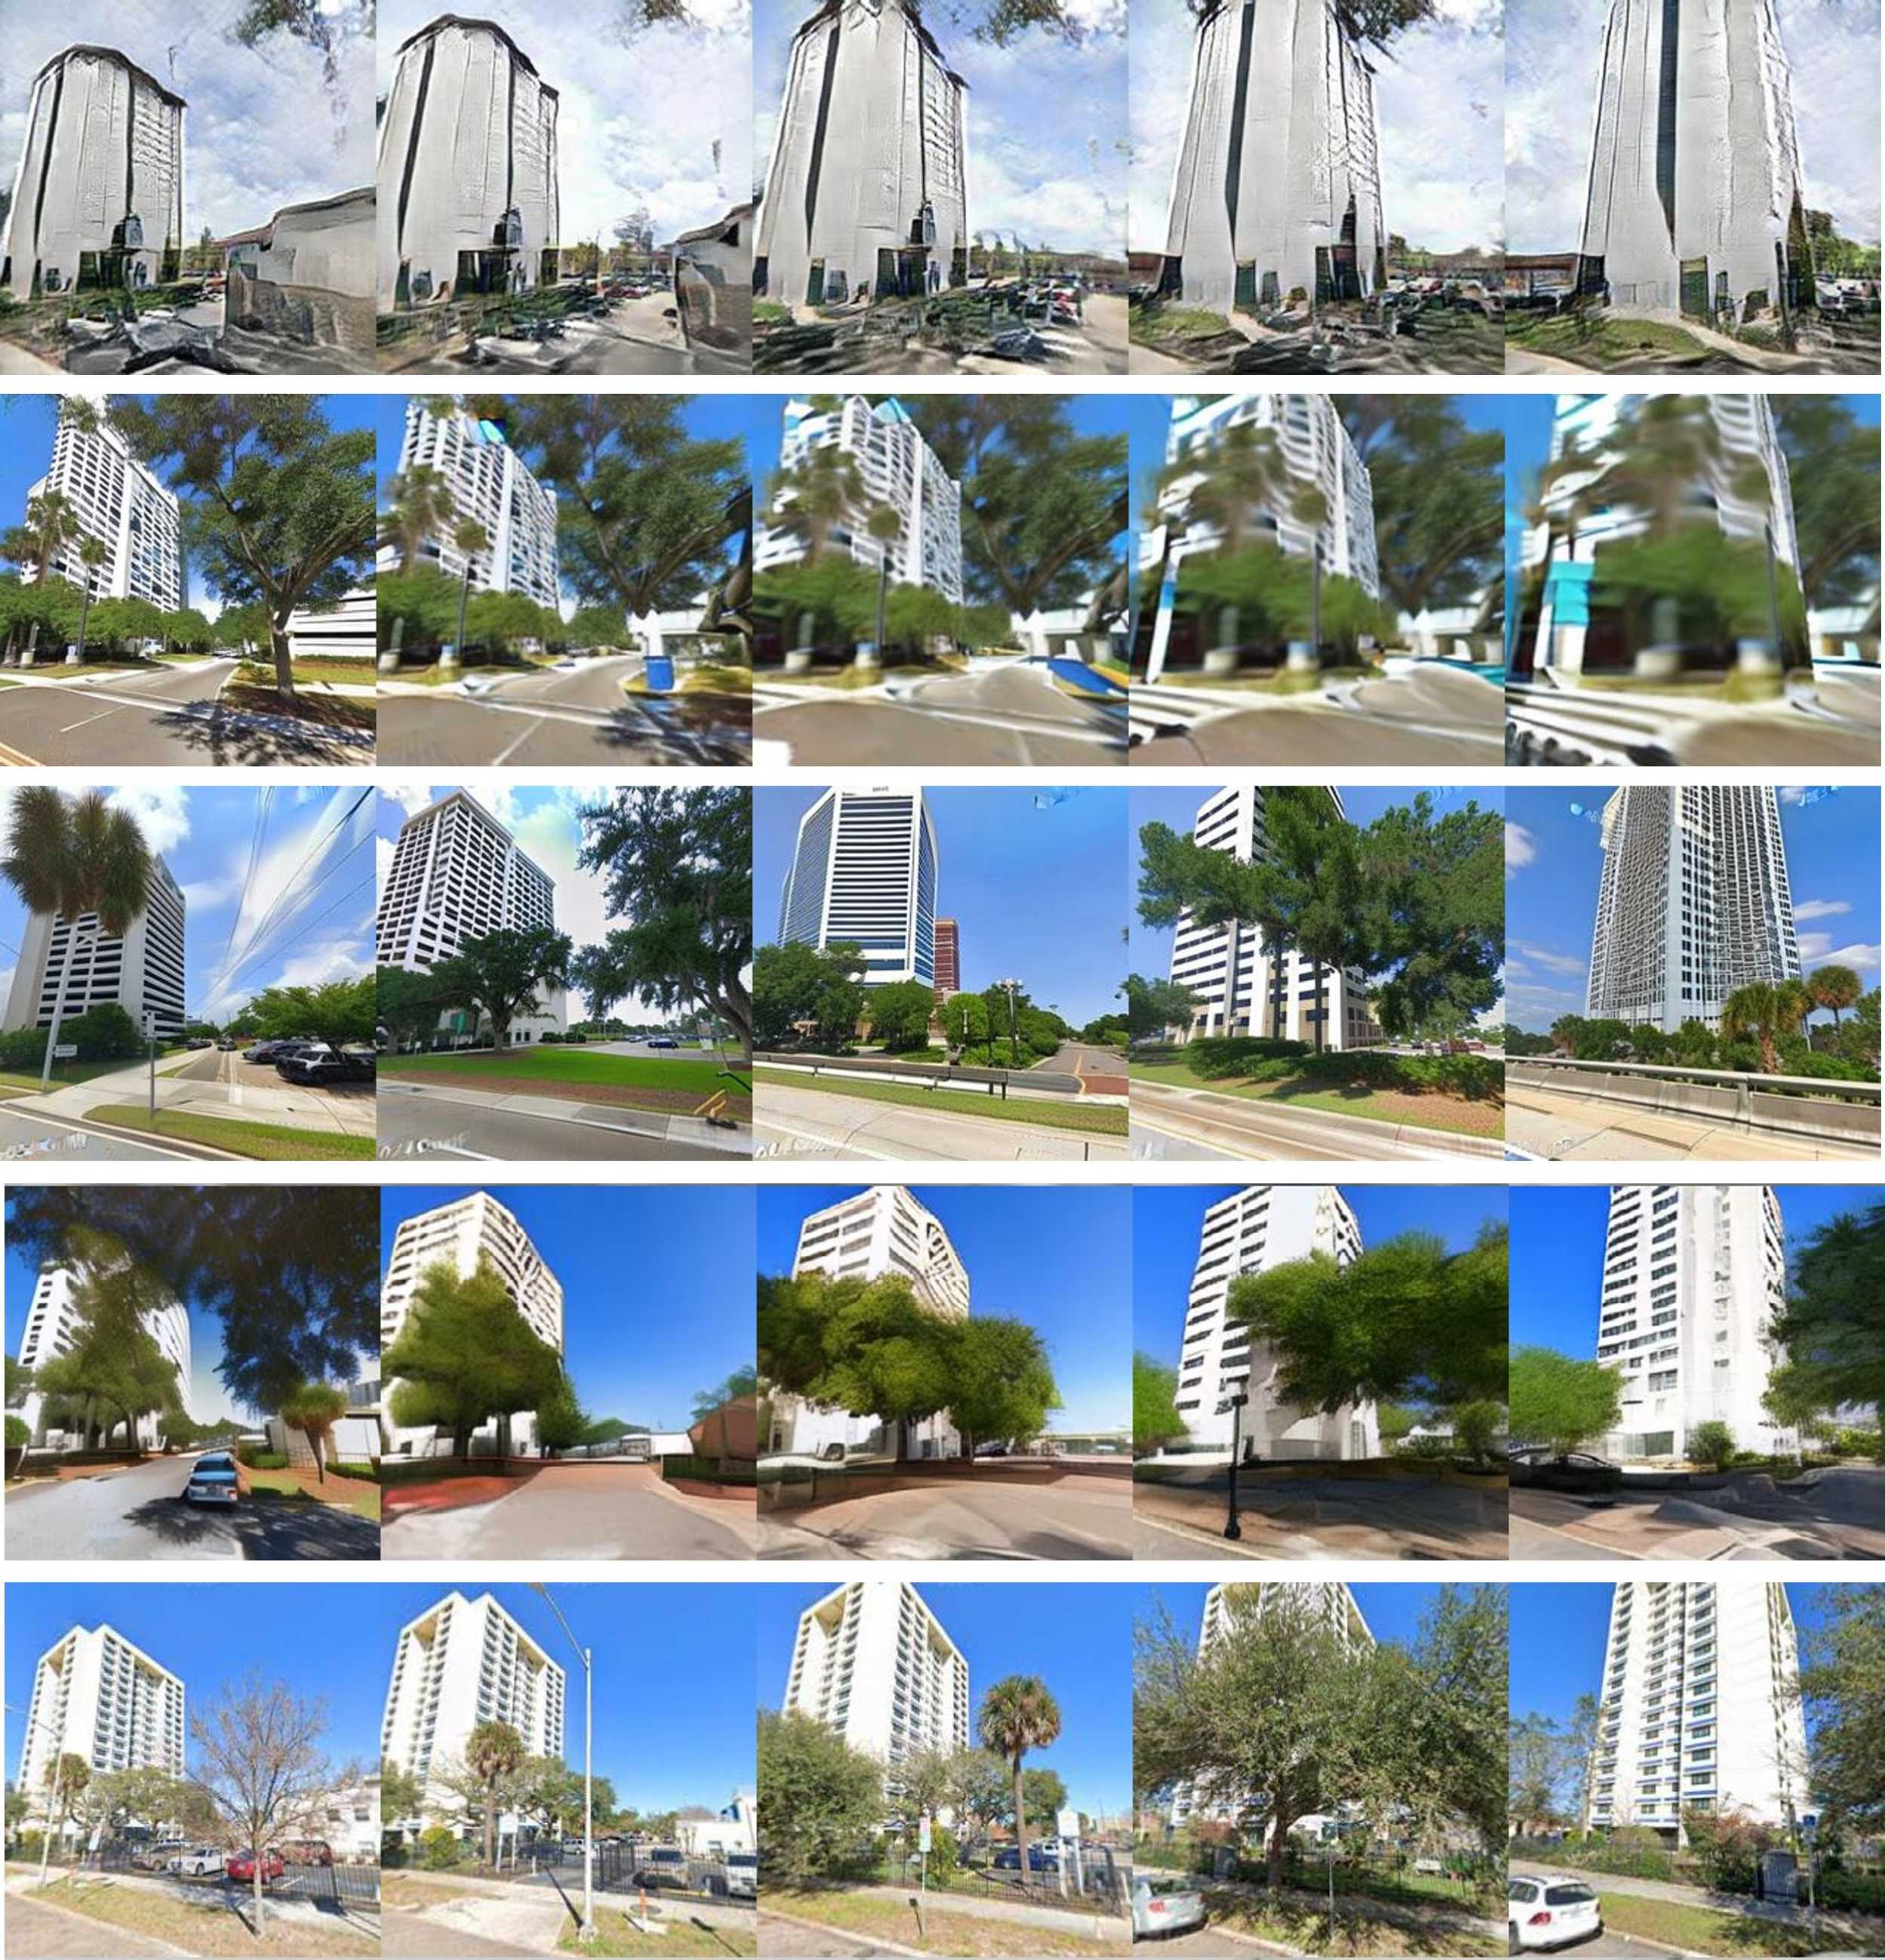}  
    \caption{Site 4}
    \end{subfigure}
    \caption{\textbf{Additional qualitative baseline comparison on the Sat2GroundScape dataset.} Our method generates more photorealistic and consistent ground views compared to the baseline methods. Notably, SceneScape \cite{Scenescape} in site 3 produces a black view due to the absence of warped content from the previous view.}
    \label{fig:supp_quali}
\end{figure*}
